# Supplementary material for: ImageRef-VL: Enabling Contextual Image Referencing in Vision-Language Models
Source: arXiv:2501.12418 source file (2025-01-20)
Supplement: Supplementary file 2 [file eval.tex]

\section{Evaluation Details}
